# Supplementary material for: Measuring density-driven errors using Kohn-Sham inversion
Source: arXiv:2004.11595 ancillary file (2020-04-24)
Supplement: Supplementary file 1 [file ksinv_supp.pdf]

# Supporting Information: Measuring density-driven errors using Kohn-Sham inversion

Seungsoo Nam,[†] Suhwan Song,[†] Eunji Sim,[*,†] and Kieron Burke[‡]

†*Department of Chemistry, Yonsei University, 50 Yonsei-ro Seodaemun-gu, Seoul 03722, Korea*

‡*Departments of Chemistry and of Physics, University of California, Irvine, CA 92697, USA*

E-mail: esim@yonsei.ac.kr

**Abstract**

Kohn-Sham inversion, that is, the finding of the exact Kohn-Sham potential for a given density, is difficult in localized basis sets. We study the precision and reliability of several inversion schemes, finding estimates of density-driven errors at a useful level of accuracy. In typical cases of substantial density-driven errors, HF-DFT is almost as accurate as DFT evaluated on CCSD(T) densities. A simple approximation in practical HF-DFT also makes errors much smaller than the density-driven errors being calculated. Two paradigm examples, stretched NaCl and the $HO{\cdot}Cl^-$ radical, illustrate just how accurate HF-DFT is.

# Contents


**1 Raw Data for Tables and Figures in the Main Text** **3**

**2 Differences Between CCSD and CCSD(T) on DFT Energy** **13**

**3 ZMP on HO·$Cl^-$ Complex** **14**

**4 Response to the Density Change for Total Energy and Energy Components** **15**

**References** **16**

# 1 Raw Data for Tables and Figures in the Main Text

Table S1: PBE energies of SC-PBE (first row) and various inversion schemes for Na, Cl atoms and NaCl molecules with Na-Cl distance $R_e$=2.4$\mathring{A}$ and $R_s$=4.5$\mathring{A}$ All energies are in Hartree. Blank cell denotes inversion did not converge.

| | | Na | Cl | NaCl($R_e$) | NaCl($R_s$) |
|---|---|---|---|---|---|
| PBE | | -162.166157 | -459.966280 | -622.281621 | -622.203130 |
| guide | $\lambda$ | ZMP | | | |
| FA | 64 | -162.162894 | -459.960943 | -622.269803 | -622.191518 |
| | 128 | -162.164113 | -459.962859 | -622.274541 | -622.196227 |
| | 256 | -162.165055 | -459.964128 | -622.277538 | -622.199154 |
| | 512 | -162.165652 | -459.965094 | -622.279558 | |
| SVWN | 64 | -162.166043 | -459.966010 | -622.281225 | -622.202742 |
| | 128 | -162.166085 | -459.966091 | -622.281351 | -622.202869 |
| | 256 | -162.166118 | -459.966157 | -622.281449 | -622.202967 |
| | 512 | -162.166138 | -459.966209 | -622.281523 | |
| BLYP | 64 | -162.166149 | -459.966247 | -622.281585 | -622.203090 |
| | 128 | -162.166152 | -459.966263 | -622.281599 | -622.203109 |
| | 256 | -162.166154 | -459.966271 | -622.281608 | -622.203118 |
| | 512 | -162.166155 | -459.966275 | -622.281613 | |
| guide | PBS | WY | | | |
| FA | D | -162.165743 | -459.964445 | -622.279813 | -622.201315 |
| | T | -162.166088 | -459.965882 | -622.281095 | -622.202794 |
| | CT | -162.166157 | -459.966262 | -622.281593 | -622.203112 |
| | CQ | -162.166156 | -459.966280 | -622.281617 | -622.203129 |
| SVWN | D | -162.166126 | -459.965937 | -622.281279 | -622.202645 |
| | T | -162.166150 | -459.966193 | -622.281497 | -622.203035 |
| | CT | -162.166156 | -459.966276 | -622.281616 | -622.203128 |
| | CQ | -162.166156 | -459.966280 | -622.281620 | -622.203130 |
| BLYP | D | -162.166145 | -459.966209 | -622.281562 | -622.203012 |
| | T | -162.166151 | -459.966269 | -622.281603 | -622.203114 |
| | CT | -162.166157 | -459.966279 | -622.281619 | -622.203128 |
| | CQ | -162.166157 | -459.966280 | -622.281621 | -622.203130 |

Table S2: Kinetic energies of SC-PBE (first row) and various inversion schemes for Na, Cl atoms and NaCl molecules with Na-Cl distance $R_e$=2.4$\AA$ and $R_s$=4.5$\AA$ All energies are in Hartree. Blank cell denotes inversion did not converge.

| | | Na | Cl | NaCl($R_e$) | NaCl($R_s$) |
|---|---|---|---|---|---|
| PBE | | 161.376820 | 458.707407 | 620.203672 | 620.013965 |
| guide | $\lambda$ | ZMP | | | |
| FA | 64 | 160.925996 | 457.652744 | 618.164101 | 617.984911 |
| | 128 | 161.049826 | 457.987823 | 618.847631 | 618.667554 |
| | 256 | 161.153764 | 458.215073 | 619.309806 | 619.127565 |
| | 512 | 161.235897 | 458.380164 | 619.634341 | |
| SVWN | 64 | 161.304965 | 458.584224 | 620.003755 | 619.814965 |
| | 128 | 161.322722 | 458.612352 | 620.050055 | 619.861166 |
| | 256 | 161.339192 | 458.635538 | 620.090499 | 619.901770 |
| | 512 | 161.352844 | 458.656183 | 620.125799 | |
| BLYP | 64 | 161.378160 | 458.702063 | 620.198719 | 620.009930 |
| | 128 | 161.378545 | 458.702413 | 620.199123 | 620.010479 |
| | 256 | 161.378161 | 458.703388 | 620.199847 | 620.011121 |
| | 512 | 161.377597 | 458.704496 | 620.200712 | |
| guide | PBS | WY | | | |
| FA | D | 161.374351 | 458.690249 | 620.187126 | 620.004458 |
| | T | 161.377145 | 458.687774 | 620.181351 | 619.995054 |
| | CT | 161.376819 | 458.707685 | 620.204233 | 620.014496 |
| | CQ | 161.376832 | 458.707306 | 620.203682 | 620.014032 |
| SVWN | D | 161.375733 | 458.699163 | 620.190737 | 620.004152 |
| | T | 161.376581 | 458.698107 | 620.190954 | 620.003537 |
| | CT | 161.376779 | 458.707442 | 620.203758 | 620.014210 |
| | CQ | 161.376827 | 458.707262 | 620.203502 | 620.014034 |
| BLYP | D | 161.376765 | 458.704679 | 620.200291 | 620.012226 |
| | T | 161.377218 | 458.704493 | 620.199844 | 620.011201 |
| | CT | 161.376830 | 458.707502 | 620.204141 | 620.014331 |
| | CQ | 161.376823 | 458.707470 | 620.203778 | 620.014255 |

Table S3: HF-PBE energies (first row) and PBE energies of various inversion schemes for Na, Cl atoms and NaCl molecules with Na-Cl distance $R_e$=2.4$\mathring{A}$ and $R_s$=4.5$\mathring{A}$ where target density is generated with HF. All energies are in Hartree.

| | | Na | Cl | NaCl($R_e$) | NaCl($R_s$) |
|---|---|---|---|---|---|
| HF | | -162.162672 | -459.958853 | -622.269770 | -622.183761 |
| guide | $\lambda$ | ZMP | | | |
| FA | 64 | -162.162317 | -459.961677 | -622.271451 | -622.185702 |
| | 128 | -162.162651 | -459.961284 | -622.272014 | -622.185927 |
| | 256 | -162.163012 | -459.960921 | -622.272300 | -622.185981 |
| | 512 | -162.163199 | -459.960779 | -622.272575 | -622.186139 |
| SVWN | 64 | -162.163896 | -459.962747 | -622.274941 | -622.188734 |
| | 128 | -162.163589 | -459.961813 | -622.273681 | -622.187323 |
| | 256 | -162.163366 | -459.961142 | -622.272854 | -622.186425 |
| | 512 | -162.163183 | -459.960644 | -622.272276 | -622.185828 |
| BLYP | 64 | -162.163910 | -459.962601 | -622.274942 | -622.188871 |
| | 128 | -162.163593 | -459.961695 | -622.273639 | -622.187356 |
| | 256 | -162.163354 | -459.961014 | -622.272754 | -622.186372 |
| | 512 | -162.163161 | -459.960495 | -622.272126 | -622.185715 |
| guide | PBS | WY | | | |
| FA | D | -162.162778 | -459.958720 | -622.270065 | -622.183308 |
| | T | -162.162961 | -459.959892 | -622.270845 | -622.184437 |
| | CT | -162.162680 | -459.959672 | -622.270512 | -622.184220 |
| | CQ | -162.162680 | -459.959009 | -622.270174 | -622.184057 |
| SVWN | D | -162.163137 | -459.960085 | -622.271437 | -622.184543 |
| | T | -162.163017 | -459.960209 | -622.271230 | -622.184680 |
| | CT | -162.162679 | -459.959685 | -622.270535 | -622.184239 |
| | CQ | -162.162679 | -459.959009 | -622.270165 | -622.184036 |
| BLYP | D | -162.163154 | -459.960335 | -622.271708 | -622.184943 |
| | T | -162.163019 | -459.960285 | -622.271338 | -622.184763 |
| | CT | -162.162680 | -459.959689 | -622.270539 | -622.184244 |
| | CQ | -162.162679 | -459.959008 | -622.270162 | -622.184034 |

Table S4: Kinetic energies of HF (first row) and inverted KS wavefunctions for Na, Cl atoms and NaCl molecules with Na-Cl distance $R_e$=2.4$\mathring{A}$ and $R_s$=4.5$\mathring{A}$ where target density is generated with HF. All energies are in Hartree.

| | | Na | Cl | NaCl($R_e$) | NaCl($R_s$) |
|---|---|---|---|---|---|
| HF | | 161.856313 | 459.470533 | 621.461140 | 621.212765 |
| guide | $\lambda$ | ZMP | | | |
| FA | 64 | 161.324167 | 458.176314 | 619.102159 | 618.864704 |
| | 128 | 161.473091 | 458.578720 | 619.878055 | 619.640409 |
| | 256 | 161.593832 | 458.855419 | 620.406975 | 620.167027 |
| | 512 | 161.688620 | 459.058941 | 620.783397 | 620.539949 |
| SVWN | 64 | 161.697618 | 459.108250 | 620.938854 | 620.688745 |
| | 128 | 161.741500 | 459.202042 | 621.075637 | 620.826437 |
| | 256 | 161.776496 | 459.273903 | 621.183054 | 620.934582 |
| | 512 | 161.804288 | 459.333344 | 621.271910 | 621.023335 |
| BLYP | 64 | 161.769544 | 459.225512 | 621.132007 | 620.882384 |
| | 128 | 161.796491 | 459.291346 | 621.223124 | 620.974580 |
| | 256 | 161.815058 | 459.341013 | 621.291190 | 621.042929 |
| | 512 | 161.828904 | 459.381138 | 621.346093 | 621.097314 |
| guide | PBS | WY | | | |
| FA | D | 161.855071 | 459.429790 | 621.425597 | 621.184012 |
| | T | 161.859887 | 459.427998 | 621.416808 | 621.171943 |
| | CT | 161.856281 | 459.471866 | 621.467274 | 621.215344 |
| | CQ | 161.856347 | 459.472183 | 621.461995 | 621.214587 |
| SVWN | D | 161.856466 | 459.439135 | 621.429605 | 621.183920 |
| | T | 161.859392 | 459.438331 | 621.426647 | 621.180792 |
| | CT | 161.856234 | 459.471624 | 621.466712 | 621.215153 |
| | CQ | 161.856346 | 459.472166 | 621.461450 | 621.213319 |
| BLYP | D | 161.857371 | 459.444627 | 621.439249 | 621.192348 |
| | T | 161.859981 | 459.444607 | 621.435349 | 621.187891 |
| | CT | 161.856285 | 459.471572 | 621.466989 | 621.215265 |
| | CQ | 161.856340 | 459.472342 | 621.461419 | 621.213260 |

Table S5: HF energies of HF wavefunctions (first row) and inverted KS wavefunctions for Na, Cl atoms and NaCl molecules with Na-Cl distance $R_e$=2.4$\AA$ and $R_s$=4.5$\AA$ where target density is generated with HF. All energies are in Hartree.

| | | Na | Cl | NaCl($R_e$) | NaCl($R_s$) |
|---|---|---|---|---|---|
| HF | | -161.858038 | -459.485969 | -621.454862 | -621.371046 |
| guide | $\lambda$ | | ZMP | | |
| FA | 64 | -161.852835 | -459.474963 | -621.434298 | -621.351527 |
| | 128 | -161.854654 | -459.478606 | -621.441651 | -621.358757 |
| | 256 | -161.856083 | -459.481112 | -621.446526 | -621.363412 |
| | 512 | -161.857060 | -459.483086 | -621.450063 | -621.366733 |
| SVWN | 64 | -161.857229 | -459.483137 | -621.451025 | -621.367777 |
| | 128 | -161.857475 | -459.483850 | -621.451854 | -621.368592 |
| | 256 | -161.857680 | -459.484443 | -621.452558 | -621.369230 |
| | 512 | -161.857835 | -459.484956 | -621.453190 | -621.369767 |
| BLYP | 64 | -161.857440 | -459.484029 | -621.452104 | -621.368710 |
| | 128 | -161.857624 | -459.484531 | -621.452665 | -621.369305 |
| | 256 | -161.857775 | -459.484922 | -621.453116 | -621.369722 |
| | 512 | -161.857890 | -459.485245 | -621.453516 | -621.370058 |
| guide | PBS | | WY | | |
| FA | D | -161.856286 | -459.480572 | -621.448219 | -621.365703 |
| | T | -161.857323 | -459.482727 | -621.451177 | -621.368590 |
| | CT | -161.858027 | -459.484798 | -621.453900 | -621.370373 |
| | CQ | -161.858028 | -459.485786 | -621.454377 | -621.370692 |
| SVWN | D | -161.857293 | -459.483113 | -621.451416 | -621.368427 |
| | T | -161.857600 | -459.483728 | -621.452380 | -621.369343 |
| | CT | -161.858026 | -459.484940 | -621.453971 | -621.370474 |
| | CQ | -161.858029 | -459.485795 | -621.454388 | -621.370712 |
| BLYP | D | -161.857340 | -459.483902 | -621.452174 | -621.369197 |
| | T | -161.857564 | -459.484194 | -621.452825 | -621.369719 |
| | CT | -161.858028 | -459.485003 | -621.453947 | -621.370491 |
| | CQ | -161.858029 | -459.485793 | -621.454390 | -621.370711 |

Table S6: PBE energy calculated with CCSD density, replacing kinetic energy part to CCSD kinetic energy (first row) and inverted KS wavefunctions for Na, Cl atoms and NaCl molecules with Na-Cl distance $R_e$=2.4$\AA$ and $R_s$=4.5$\AA$ where target density is generated with CCSD. All energies are in Hartree.

| | | Na | Cl | NaCl($R_e$) | NaCl($R_s$) |
|---|---|---|---|---|---|
| CCSD | | -162.154762 | -459.802744 | -622.084180 | -622.002597 |
| guide | $\lambda$ | ZMP | | | |
| FA | 64 | -162.163202 | -459.962519 | -622.272309 | -622.187455 |
| | 128 | -162.163879 | -459.963298 | -622.274795 | -622.189548 |
| | 256 | -162.164401 | -459.963780 | -622.276307 | -622.190787 |
| | 512 | -162.164650 | -459.964201 | -622.277280 | -622.191612 |
| SVWN | 64 | -162.165090 | -459.965089 | -622.278610 | -622.193298 |
| | 128 | -162.164927 | -459.964755 | -622.278108 | -622.192601 |
| | 256 | -162.164782 | -459.964526 | -622.277758 | -622.192140 |
| | 512 | -162.164647 | -459.964345 | -622.277458 | -622.191790 |
| BLYP | 64 | -162.165075 | -459.965115 | -622.278707 | -622.193517 |
| | 128 | -162.164881 | -459.964749 | -622.278104 | -622.192659 |
| | 256 | -162.164721 | -459.964467 | -622.277662 | -622.192081 |
| | 512 | -162.164590 | -459.964239 | -622.277303 | -622.191663 |
| guide | PBS | WY | | | |
| FA | D | -162.164143 | -459.962294 | -622.275294 | -622.189364 |
| | T | -162.164246 | -459.963563 | -622.276296 | -622.190674 |
| | CT | -162.164104 | -459.963487 | -622.276118 | -622.190366 |
| | CQ | -162.163816 | -459.963374 | -622.275858 | -622.190068 |
| SVWN | D | -162.164510 | -459.963687 | -622.276690 | -622.190619 |
| | T | -162.164307 | -459.963878 | -622.276691 | -622.190918 |
| | CT | -162.164106 | -459.963501 | -622.276146 | -622.190379 |
| | CQ | -162.163463 | -459.963374 | -622.275850 | -622.190075 |
| BLYP | D | -162.164527 | -459.963948 | -622.276964 | -622.191022 |
| | T | -162.164309 | -459.963954 | -622.276800 | -622.191001 |
| | CT | -162.164106 | -459.963503 | -622.276153 | -622.190381 |
| | CQ | -162.163808 | -459.963374 | -622.275851 | -622.190045 |

Table S7: CCSD kinetic energy (first row) and inverted KS wavefunctions for Na, Cl atoms and NaCl molecules with Na-Cl distance $R_e$=2.4Å and $R_s$=4.5Å where target density is generated with CCSD. All energies are in Hartree.

| | | Na | Cl | NaCl($R_e$) | NaCl($R_s$) |
|---|---|---|---|---|---|
| CCSD | | 161.856313 | 459.470533 | 621.461140 | 621.212765 |
| guide | $\lambda$ | | ZMP | | |
| FA | 64 | 161.190657 | 457.942576 | 618.737372 | 618.525569 |
| | 128 | 161.338172 | 458.324065 | 619.490355 | 619.278413 |
| | 256 | 161.460657 | 458.589221 | 620.008974 | 619.794399 |
| | 512 | 161.557411 | 458.787264 | 620.381773 | 620.163374 |
| SVWN | 64 | 161.565474 | 458.874060 | 620.573536 | 620.348977 |
| | 128 | 161.607536 | 458.947380 | 620.688001 | 620.464375 |
| | 256 | 161.643847 | 459.007935 | 620.785393 | 620.562216 |
| | 512 | 161.673335 | 459.061892 | 620.870584 | 620.647050 |
| BLYP | 64 | 161.637776 | 458.991415 | 620.767144 | 620.543116 |
| | 128 | 161.662739 | 459.036829 | 620.835847 | 620.612899 |
| | 256 | 161.682487 | 459.075187 | 620.893773 | 620.670834 |
| | 512 | 161.697978 | 459.109784 | 620.944925 | 620.721195 |
| guide | PBS | | WY | | |
| FA | D | 161.723560 | 459.157635 | 621.023077 | 620.805357 |
| | T | 161.729026 | 459.155433 | 621.017368 | 620.796083 |
| | CT | 161.724757 | 459.196923 | 621.064894 | 620.836020 |
| | CQ | 161.726105 | 459.196298 | 621.060448 | 620.834960 |
| SVWN | D | 161.725079 | 459.166925 | 621.026975 | 620.805125 |
| | T | 161.728587 | 459.165766 | 621.027209 | 620.804894 |
| | CT | 161.724807 | 459.196696 | 621.064224 | 620.835701 |
| | CQ | 161.726691 | 459.196583 | 621.060318 | 620.834881 |
| BLYP | D | 161.726056 | 459.172452 | 621.036676 | 620.813613 |
| | T | 161.729196 | 459.172150 | 621.035991 | 620.812131 |
| | CT | 161.724754 | 459.196770 | 621.064512 | 620.835756 |
| | CQ | 161.726104 | 459.196768 | 621.060294 | 620.834947 |

Table S8: PBE energies of Na, Cl atoms and NaCl molecules with various Na-Cl distances (in Å). All energies are in Hartree.

| | CCSD(T) | PBE | HF-PBE | DC-PBE[HF] | DC-PBE[CC] |
|---|---|---|---|---|---|
| Na | -161.870227 | -162.166157 | -162.162672 | -162.162680 | -162.164104 |
| Cl | -459.708617 | -459.966280 | -459.958853 | -459.959671 | -459.963487 |
| 2.0 | -621.705182 | -622.252420 | -622.240597 | -622.241506 | -622.247205 |
| 2.1 | -621.720444 | -622.267868 | -622.256108 | -622.256978 | -622.262603 |
| 2.2 | -621.729030 | -622.276626 | -622.264873 | -622.265709 | -622.271304 |
| 2.3 | -621.732846 | -622.280727 | -622.268941 | -622.269734 | -622.275327 |
| 2.4 | -621.733434 | -622.281621 | -622.269770 | -622.270512 | -622.276118 |
| 2.5 | -621.731965 | -622.280335 | -622.268389 | -622.269085 | -622.274720 |
| 2.6 | -621.729190 | -622.277588 | -622.265521 | -622.266179 | -622.271852 |
| 2.7 | -621.725518 | -622.273881 | -622.261669 | -622.262289 | -622.268020 |
| 2.8 | -621.721189 | -622.269567 | -622.257185 | -622.257795 | -622.263566 |
| 2.9 | -621.716397 | -622.264896 | -622.252324 | -622.252907 | -622.258751 |
| 3.0 | -621.711319 | -622.260050 | -622.247265 | -622.247831 | -622.253731 |
| 3.1 | -621.706103 | -622.255154 | -622.242133 | -622.242686 | -622.248651 |
| 3.2 | -621.700866 | -622.250299 | -622.237020 | -622.237559 | -622.243574 |
| 3.3 | -621.695689 | -622.245546 | -622.231984 | -622.232510 | -622.238573 |
| 3.4 | -621.690630 | -622.240938 | -622.227067 | -622.227585 | -622.233680 |
| 3.5 | -621.685724 | -622.236503 | -622.222296 | -622.222795 | -622.228931 |
| 3.6 | -621.680995 | -622.232261 | -622.217686 | -622.218187 | -622.224337 |
| 3.7 | -621.676455 | -622.228220 | -622.213245 | -622.213733 | -622.219910 |
| 3.8 | -621.672111 | -622.224386 | -622.208979 | -622.209456 | -622.215654 |
| 3.9 | -621.667963 | -622.220760 | -622.204886 | -622.205364 | -622.211565 |
| 4.0 | -621.664008 | -622.217342 | -622.200965 | -622.201441 | -622.207644 |
| 4.1 | -621.660243 | -622.214123 | -622.197210 | -622.197685 | -622.203879 |
| 4.2 | -621.656660 | -622.211101 | -622.193619 | -622.194084 | -622.200283 |
| 4.3 | -621.653250 | -622.208267 | -622.190184 | -622.190649 | -622.196839 |
| 4.4 | -621.650003 | -622.205612 | -622.186899 | -622.187361 | -622.193538 |
| 4.5 | -621.646909 | -622.203130 | -622.183761 | -622.184219 | -622.190366 |
| 4.6 | -621.643957 | -622.200812 | -622.180763 | -622.181221 | -622.187352 |
| 4.7 | -621.641139 | -622.198648 | -622.177898 | -622.178353 | -622.184458 |
| 4.8 | -621.638446 | -622.196636 | -622.175168 | -622.175619 | -622.181682 |
| 4.9 | -621.635870 | -622.194757 | -622.172556 | -622.173005 | -622.179031 |
| 5.0 | -621.633403 | -622.192987 | -622.170042 | -622.170489 | -622.176477 |
| 5.1 | -621.631041 | -622.191330 | -622.167631 | -622.168076 | -622.174030 |
| 5.2 | -621.628777 | -622.189792 | -622.165332 | -622.165774 | -622.171681 |
| 5.3 | -621.626606 | -622.188358 | -622.163131 | -622.163570 | -622.169439 |
| 5.4 | -621.624524 | -622.187009 | -622.161013 | -622.161449 | -622.167272 |
| 5.5 | -621.622526 | -622.185749 | -622.158982 | -622.159421 | -622.165198 |
| 5.6 | -621.620608 | -622.184580 | -622.157043 | -622.157478 | -622.163213 |
| 5.7 | -621.618766 | -622.183489 | -622.155184 | -622.155616 | -622.161307 |
| 5.8 | -621.616995 | -622.182457 | -622.153389 | -622.153820 | -622.159467 |

**Table S8 continued from previous page**

| | CCSD(T) | PBE | HF-PBE | DC-PBE[HF] | DC-PBE[CC] |
|---|---|---|---|---|---|
| 5.9 | -621.615292 | -622.181485 | -622.151658 | -622.152089 | -622.157691 |
| 6.0 | -621.613654 | -622.180580 | -622.150000 | -622.150428 | -622.155991 |
| 6.1 | -621.612077 | -622.179739 | -622.148412 | -622.148839 | -622.154361 |
| 6.2 | -621.610558 | -622.178950 | -622.146885 | -622.147312 | -622.152790 |
| 6.3 | -621.609094 | -622.178197 | -622.145402 | -622.145828 | -622.151269 |
| 6.4 | -621.607681 | -622.177483 | -622.143966 | -622.144391 | -622.149794 |
| 6.5 | -621.606319 | -622.176815 | -622.142586 | -622.143009 | -622.148375 |
| 6.6 | -621.605002 | -622.176194 | -622.141263 | -622.141685 | -622.147020 |
| 6.7 | -621.603731 | -622.175611 | -622.139989 | -622.140410 | -622.145720 |
| 6.8 | -621.602501 | -622.175059 | -622.138757 | -622.139175 | -622.144452 |
| 6.9 | -621.601311 | -622.174529 | -622.137558 | -622.137979 | -622.143225 |
| 7.0 | -621.600159 | -622.174018 | -622.136387 | -622.136807 | -622.142021 |
| 7.1 | -621.599042 | -622.173533 | -622.135254 | -622.135672 | -622.140865 |
| 7.2 | -621.597960 | -622.173081 | -622.134162 | -622.134578 | -622.139749 |
| 7.3 | -621.596910 | -622.172660 | -622.133114 | -622.133528 | -622.138685 |
| 7.4 | -621.595891 | -622.172263 | -622.132103 | -622.132515 | -622.137655 |
| 7.5 | -621.594901 | -622.171883 | -622.131119 | -622.131537 | -622.136650 |
| 7.6 | -621.593939 | -622.171514 | -622.130158 | -622.130570 | -622.135662 |
| 7.7 | -621.593004 | -622.171155 | -622.129217 | -622.129633 | -622.134700 |
| 7.8 | -621.592094 | -622.170807 | -622.128296 | -622.128709 | -622.133763 |
| 7.9 | -621.591208 | -622.170468 | -622.127393 | -622.127804 | -622.132857 |
| 8.0 | -621.590346 | -622.170144 | -622.126513 | -622.126929 | -622.131963 |

Table S9: PBE energies of OH, $Cl^-$ and linear $HO{\cdot}Cl^-$ complex with various H-Cl distances (in $\AA$). All energies are in Hartree.

| | CCSD(T) | PBE | HF-PBE | DC-PBE[HF] | DC-PBE[CC] |
|---|---|---|---|---|---|
| OH | -75.658331 | -75.682384 | -75.673990 | -75.674850 | -75.680453 |
| Cl | -459.837402 | -460.100583 | -460.093117 | -460.093383 | -460.097317 |
| 1.50 | -535.500638 | -535.790611 | -535.768178 | -535.771453 | -535.783120 |
| 1.60 | -535.512822 | -535.802796 | -535.780589 | -535.783654 | -535.795098 |
| 1.70 | -535.520381 | -535.810449 | -535.788336 | -535.791207 | -535.802471 |
| 1.80 | -535.524798 | -535.815050 | -535.792911 | -535.795612 | -535.806716 |
| 1.85 | -535.526158 | -535.816535 | -535.794340 | -535.796953 | -535.807992 |
| 1.90 | -535.527082 | -535.817609 | -535.795329 | -535.797863 | -535.808835 |
| 1.95 | -535.527650 | -535.818352 | -535.795959 | -535.798401 | -535.809320 |
| 2.00 | -535.527924 | -535.818828 | -535.796295 | -535.798666 | -535.809519 |
| 2.05 | -535.527959 | -535.819094 | -535.796393 | -535.798665 | -535.809489 |
| 2.10 | -535.527799 | -535.819193 | -535.796299 | -535.798515 | -535.809263 |
| 2.15 | -535.527482 | -535.819164 | -535.796053 | -535.798208 | -535.808901 |
| 2.20 | -535.527038 | -535.819038 | -535.795687 | -535.797754 | -535.808418 |
| 2.30 | -535.525872 | -535.818589 | -535.794695 | -535.796659 | -535.807210 |

Table S9 continued from previous page

| | CCSD(T) | PBE | HF-PBE | DC-PBE[HF] | DC-PBE[CC] |
|---|---|---|---|---|---|
| 2.40 | -535.524468 | -535.817995 | -535.793486 | -535.795355 | -535.805807 |
| 2.50 | -535.522941 | -535.817350 | -535.792169 | -535.793948 | -535.804314 |
| 2.60 | -535.521373 | -535.816713 | -535.790817 | -535.792507 | -535.802796 |
| 2.70 | -535.519818 | -535.816118 | -535.789477 | -535.791108 | -535.801319 |
| 2.80 | -535.518312 | -535.815585 | -535.788178 | -535.789738 | -535.799891 |
| 2.90 | -535.516879 | -535.815121 | -535.786937 | -535.788448 | -535.798534 |
| 3.00 | -535.515529 | -535.814728 | -535.785765 | -535.787216 | -535.797258 |
| 3.10 | -535.514271 | -535.814405 | -535.784665 | -535.786072 | -535.796066 |
| 3.20 | -535.513104 | -535.814146 | -535.783639 | -535.784996 | -535.794948 |
| 3.30 | -535.512026 | -535.813947 | -535.782684 | -535.784003 | -535.793929 |
| 3.40 | -535.511035 | -535.813802 | -535.781797 | -535.783085 | -535.792966 |
| 3.50 | -535.510124 | -535.813703 | -535.780975 | -535.782232 | -535.792080 |
| 3.60 | -535.509288 | -535.813645 | -535.780213 | -535.781443 | -535.791272 |
| 3.70 | -535.508522 | -535.813624 | -535.779506 | -535.780708 | -535.790511 |
| 3.80 | -535.507818 | -535.813633 | -535.778852 | -535.780034 | -535.789820 |
| 3.90 | -535.507172 | -535.813669 | -535.778244 | -535.779407 | -535.789166 |
| 4.00 | -535.506578 | -535.813729 | -535.777681 | -535.778831 | -535.788579 |
| 4.10 | -535.506029 | -535.813808 | -535.777159 | -535.778304 | -535.788022 |
| 4.20 | -535.505523 | -535.813904 | -535.776673 | -535.777805 | -535.787515 |
| 4.30 | -535.505054 | -535.814014 | -535.776221 | -535.777356 | -535.787036 |
| 4.40 | -535.504618 | -535.814135 | -535.775801 | -535.776926 | -535.786600 |
| 4.50 | -535.504213 | -535.814267 | -535.775409 | -535.776529 | -535.786185 |
| 4.60 | -535.503835 | -535.814406 | -535.775043 | -535.776161 | -535.785813 |
| 4.70 | -535.503482 | -535.814552 | -535.774701 | -535.775818 | -535.785453 |
| 4.80 | -535.503152 | -535.814703 | -535.774381 | -535.775492 | -535.785126 |
| 4.90 | -535.502843 | -535.814858 | -535.774082 | -535.775198 | -535.784812 |
| 5.00 | -535.502554 | -535.815016 | -535.773801 | -535.774914 | -535.784539 |
| 5.10 | -535.502282 | -535.815177 | -535.773538 | -535.774656 | -535.784260 |
| 5.20 | -535.502027 | -535.815340 | -535.773290 | -535.774403 | -535.784014 |
| 5.30 | -535.501787 | -535.815504 | -535.773058 | -535.774174 | -535.783773 |
| 5.40 | -535.501561 | -535.815668 | -535.772838 | -535.773951 | -535.783547 |
| 5.50 | -535.501348 | -535.815832 | -535.772631 | -535.773747 | -535.783342 |
| 5.60 | -535.501147 | -535.815996 | -535.772436 | -535.773554 | -535.783139 |
| 5.70 | -535.500957 | -535.816160 | -535.772251 | -535.773356 | -535.782955 |
| 5.80 | -535.500777 | -535.816322 | -535.772075 | -535.773193 | -535.782777 |

# 2 Differences Between CCSD and CCSD(T) on DFT Energy

Table S10: PBE energy calculated with inverted KS wavefunctions for Na, Cl atoms and NaCl molecules with Na-Cl distance $R_e$=2.4$\AA$ and $R_s$=4.5$\AA$ where target density is generated with CCSD(T). All energies are in Hartree.

| guide | PBS | Na | Cl | NaCl($R_e$) | NaCl($R_s$) |
|---|---|---|---|---|---|
| FA | D | -162.164099 | -459.962287 | -622.275314 | -622.189433 |
| | T | -162.164205 | -459.963553 | -622.276329 | -622.190763 |
| | CT | -162.164064 | -459.963487 | -622.276137 | -622.190463 |
| | CQ | -162.163697 | -459.963378 | -622.275852 | -622.190219 |
| SVWN | D | -162.164468 | -459.963685 | -622.276722 | -622.190703 |
| | T | -162.164266 | -459.963869 | -622.276731 | -622.191009 |
| | CT | -162.164064 | -459.963498 | -622.276159 | -622.190492 |
| | CQ | -162.163424 | -459.963378 | -622.275848 | -622.190212 |
| BLYP | D | -162.164486 | -459.963944 | -622.277001 | -622.191105 |
| | T | -162.164266 | -459.963945 | -622.276840 | -622.191089 |
| | CT | -162.164064 | -459.963501 | -622.276164 | -622.190495 |
| | CQ | -162.163764 | -459.963377 | -622.275846 | -622.190210 |

Table S11: First row shows Na-Cl binding energy using CCSD, CCSD(T), and their differences($\Delta$(T)) . The difference between CCSD and CCSD(T) is approximately 2 kcal/-mol. On the other hand, the second and third-row shows inversion results calculated on PBE functional, where the guiding potential is FA or BLYP. In this case, the difference between CCSD and CCSD(T) density is similar to or less than 0.1 kcal/mol. Thus, although CCSD and CCSD(T) show some differences, their density may be similar to each other. Inversions were performed with WY/CT. All energies are in kcal/mol.

| | $E_{rxn}(R_e)$ | | | $E_{rxn}(R_s)$ | | |
|---|---|---|---|---|---|---|
| | CCSD | CCSD(T) | $\Delta$(T) | CCSD | CCSD(T) | $\Delta$(T) |
| wfn | -94.96 | -97.00 | -2.04 | -40.41 | -42.71 | -2.30 |
| FA | -93.20 | -93.24 | -0.04 | -39.39 | -39.48 | -0.09 |
| BLYP | -93.21 | -93.25 | -0.03 | -39.39 | -39.49 | -0.10 |

# 3 ZMP on HO·Cl$^-$ Complex

Although we claim that the uncertainty of inversion 0.5 kcal/mol on the NaCl example, we observed that uncertainty of inversion at another system, i.e., HO·Cl$^-$ complex, is also less than 0.5 kcal/mol.

Table S12: PBE energies of OH, Cl$^-$, HO·Cl$^-$(H-Cl distance 2$\AA$), and their differences ($E_{rxn}$) using inversions. For WY, we used FA guiding potential and aug-cc-pCVTZ potential basis set. For ZMP, we used FA or BLYP guiding potential and $\lambda$=512. For both HF and CCSD target density, the inversions show deviations less than 0.5 kcal/mol. All energies are in Hartree, except $E_{rxn}$.

| | WY/FA | ZMP/FA | ZMP/BLYP |
|---|---|---|---|
| | | HF | |
| OH | -75.674850 | -75.676276 | -75.675798 |
| Cl$^-$ | -460.093383 | -460.094722 | -460.094503 |
| HO·Cl$^-$ | -535.798666 | -535.801816 | -535.800891 |
| $E_{rxn}$(kcal/mol) | -19.10 | -19.34 | -19.20 |
| | | CCSD | |
| OH | -75.680453 | -75.681203 | -75.681002 |
| Cl$^-$ | -460.097317 | -460.098047 | -460.098100 |
| HO·Cl$^-$ | -535.809519 | -535.811057 | -535.810805 |
| $E_{rxn}$(kcal/mol) | -19.92 | -19.96 | -19.89 |

# 4 Response to the Density Change for Total Energy and Energy Components

Generally, total energies are much less sensitive to the density change than energy components, as can be seen in the differences between Table S1 and S2. (Inversion error can be regarded as density change from SC-PBE density.) This means energy components cancel out each other to reproduce much smaller energy differences than individual components. The reason for this cancellation becomes obvious when considering the functional expansion.[1] For two densities $n'(\mathbf{r})$ and $n''(\mathbf{r})$ that slightly differ by $\Delta n(\mathbf{r}) = n''(\mathbf{r}) - n'(\mathbf{r})$ and arbitrary density functional $X[n]$, we can write the functional difference $X[n''] - X[n']$ as

$$X[n''] - X[n'] = \int d\mathbf{r} \frac{\delta X[n]}{\delta n(\mathbf{r})}\Big|_{n'} \Delta n(\mathbf{r}) + \frac{1}{2} \iint d\mathbf{r}_1 d\mathbf{r}_2 \frac{\delta^2 X[n](\mathbf{r})}{\delta n(\mathbf{r}_1)\delta n(\mathbf{r}_2)}\Big|_{n'} \Delta n(\mathbf{r}_1)\Delta n(\mathbf{r}_2) + .... \quad (1)$$

If $n'$ does not define minimum or maximum of $X[n]$, the first term (in the order of $\Delta n$) dominates the functional difference. On the other hand, if functional $Y[n]$ delivers a minimum or maximum at $n = n'$,

$$\frac{\delta Y[n]}{\delta n(\mathbf{r})}\Big|_{n'} = 0, \quad (2)$$

and thus

$$Y[n''] - Y[n'] = \frac{1}{2} \iint d\mathbf{r}_1 d\mathbf{r}_2 \frac{\delta^2 Y[n]}{\delta n(\mathbf{r}_1)\delta n(\mathbf{r}_2)}\Big|_{n'} \Delta n(\mathbf{r}_1)\Delta n(\mathbf{r}_2) + ..., \quad (3)$$

which shows that the functional difference is in the order of $\Delta n^2$.

For electron density from any reasonable procedure (HF, DFT, or any *ab initio* calculations) does not differ dramatically. Therefore, Eq. S2 is roughly satisfied for any (reasonable) total energy functionals even for densities that are not strictly variational minimum. On the other hand, these densities are far from a variational minimum of specific energy component functionals, and Eq. S2 is nonzero. (For example, density of free particles in case of kinetic energy functional.) Thus, energy components are much more sensitive (order of $\Delta n$) than total energy (order of $\Delta n^2$) for the same density change.

# References

(1) Ernzerhof, M. Taylor-series expansion of density functionals. *Physical Review A* **1994**, *50*, 4593.
